# Supplementary material for: On the KL-Divergence-based Robust Satisficing Model
Source: arXiv:2408.09157 source file (2024-08-17)
Supplement: Supplementary file 1 [file appendix.tex]

\appendix
\section{Additional discussion}
When the true distribution $\Popt$ is a discrete distribution with $K$
supports e.g. $\{z_{k}\}_{k\in[K]}$. In this case, we use $\Pemp_{k}=\frac{N_{k}}{N}$
to denote empirical distribution where $N_{K}$ is the number of symbol $z_{k}$
in samples.

We can not obtain a finite sample guarantee through the same method 
as \ref{thm: asymptotic discrete} and \ref{thm: asymptotic continuous}.
The main reason is that finite sample guarantees relies on concentration 
inequalities with respect to $\mathbb{E}_{\mathbb{P}^{N}}[D_{KL}(\Popt\Vert\Pemp)]$. However, 
$D_{KL}(\Popt, \Pemp)$ can be unbounded since $\Pemp_{k}$ can be zero for 
some $k\in\{K\}$ which results $\mathbb{E}_{\mathbb{P}^{N}}[D_{KL}(\Popt\Vert\Pemp)]$ being
not well-defined. If we consider the event $\{\Pemp_{k}\neq 0, \forall
k\in[K], \tbz\sim\Popt\}$, then the sample process can not be i.i.d which violates the general assumption of i.i.d. sampling in concentration inequalities.
One of possible methods to address this issue by adopting Laplace estimator to replace $\Pemp$.
Laplace estimator is defined as following:
\begin{equation}
\Pemp_{k}^{l}=\frac{N_{k}+1}{N+k}, \forall k\in[K].
\end{equation}
$\Pemp^{l}$ adds one sample for any support point to avoid 
unbounded $D_{KL}(\Popt\Vert\Pemp^{l})$. According to the recent advances in 
KL divergence\cite{canonne2023concentration}, we have 

\begin{theorem}
With probability at least $1-\delta$, $D_{KL}(\Popt\Vert\Pemp^{l})$ is
upper bounded by 
\begin{equation}
    \mathbb{E}_{\mathbb{P}^{N}}[D_{KL}(\Popt\Vert\Pemp^{l})]+
    \frac{6\sqrt{K\log^{5}(4K/\delta)}}{N}+\frac{311}{N}+
    \frac{160K}{N^{3/2}}.
\end{equation}
\end{theorem}
Therefore, we use $\Pemp^{l}$ to replace the $\Pemp$ in \eqref{Prob: 
klrs Sim}, we have the following formulation:
\begin{equation}\label{Prob: klrs Lap}
  \begin{aligned}
\min_{\lambda\geq 0, \bt\in\Theta} & \quad \lambda\\
\text{s.t.} \quad & \quad \hat{R}^{l}(\bt, \lambda) \leq \tau,
  \end{aligned}
  \end{equation}
with $\hat{R}^{l}(\bt, \lambda)\triangleq\lambda\log
\left(\mathbb{E}_{\Pemp^{l}}
      \left[\exp\left(l(\bt, \tbz)/\lambda\right)
      \right]\right)$. Then the optimizer of 
\eqref{Prob: klrs Lap} enjoys the following finite sample performance 
guarantee, 

\begin{theorem}
Suppose that $\Popt$ is a discrete distribution supported by $K$ points.
For every optimal solution $(\bt^{\ast}_{N}, \lambda^{\ast}_{N})$ of 
\eqref{Prob: klrs Lap} and a given $r\geq \mathbb{E}[D(\Popt\Vert\Pemp^{l})]
+\frac{311}{N}+\frac{160k}{N^{3/2}}$, with probability at least
$1-\delta$, 
\begin{equation}
\mathbb{E}_{\Popt}[l(\bt_{N}^{\ast}, \tbz)]\leq \tau+
\lambda_{N}^{\ast}r,
\end{equation}
where $\delta=4K\exp(-\sqrt[5]{\frac{1}{36K}(Nr-N\mathbb{E}_{\mathbb{P}^{N}}
[D(\Popt\Vert\Pemp^{l})]-311-\frac{160K}{\sqrt{N}})^{2}})$.
\end{theorem}
This performance guarantee does not hold for any non-negative $r$ because Laplace estimator $\Pemp^{l}$ is a biased estimation for $\Popt$. The Laplace estimator adds an extra sample to each support point, effectively superimposing a uniform distribution on $\Popt$. The support points with high probability will be underestimated while the probability of other points will be overestimated by $\Pemp^{l}$.

\section{Proofs and Details for Section\ref{sec: model}}
\paragraph{Proof of Proposition \ref{thm: eq} and Proposition \ref{prop: optDistn}}

  Problem \eqref{Prob: rs} is equivalent to the following formulation:
  \begin{equation}
      \begin{aligned}
          &\inf_{\bt\in\Theta, \lambda\geq 0}\lambda\\
          &\text{s.t.}\sup_{\mathbb{P}\ll\hat{\mathbb{P}}}\{
            \mathbb{E}_{\mathbb{P}}[l(\bt, \tbz)]-\lambda D(\mathbb{P}
            \Vert \hat{\mathbb{P}})\}\leq \tau,   \quad \forall \bP \in 
            \{\mathbb{P}_0 \in \Pset(\Omega): \mathbb{P}_0\ll
          \Pemp\}.
      \end{aligned}
  \end{equation}

  \cite{follmer2002convex, shapiro2021lectures, 
  follmer2011stochastic} provides dual formulation for the left hand 
  expression of the constraint. For further analysis convenience, 
  We will write the algebraic transformations after duality below.
  \begin{equation}
    \begin{aligned}
    &\sup_{\mathbb{P}\ll\hat{\mathbb{P}}}\{\mathbb{E}_{\mathbb{P}}[l(\tbz,  
    \bt)]-\lambda D(\mathbb{P}\Vert \hat{\mathbb{P}})\}\\
  =&\inf_{\eta}\sup_{\mathbb{P}}\{\mathbb{E}_{\mathbb{P}}[l(f(\bt, \tbz))]-\lambda
  \mathbb{E}_{\mathbb{P}}[\phi(\frac{d\mathbb{P}}{d\Pemp})]
  +\eta-\eta\mathbb{E}_{\mathbb{P}}[1]\}\\
  =&\inf_{\eta}\{\eta+\mathbb{E}_{\hat{\mathbb{P}}}\sup_{\mathbb{P}}\{l(\bt, \tbz)
  \frac{d\mathbb{P}}{d\mathbb{\hat{\mathbb{P}}}}-\eta\frac{d\mathbb{P}}
  {d\mathbb{\hat{\mathbb{P}}}}-\lambda\frac{\mathbb{P}}{\Pemp}\phi(\frac{d\mathbb{P}}{d\hat{\mathbb{P}}})\}\}\\
  =&\inf_{\eta}\{\eta+\mathbb{E}_{\hat{\mathbb{P}}}\left[(\lambda\phi)^{\ast}
    (l(\bt, \tbz)-\eta)\right]\}\\
  =&\inf_{\eta}\{\eta+\lambda\mathbb{E}_{\hat{\mathbb{P}}}\left[\phi^{\ast}
  (\frac{l(\bt, \tbz)-\eta}{\lambda})\right]\},
    \end{aligned}
  \end{equation}

  where $\eta$ is dual variable for constraint $\mathbb{E}_{\mathbb{P}}[1]=1$. 
  Recall that $\phi(t)=t\log(t)-t+1$ in 
  Definition \ref{Dist: KL}. $\phi^{\ast}(s)$ is the conjugate function of 
  $\phi(t)$, where $\phi^{\ast}(s)\triangleq\displaystyle{\sup_{t}}\{ts-\phi(t)\}=
  \exp(s)-1$ and the corresponding optimizer is $t=\exp(s)$. And $(\lambda\phi)^{\ast}=\lambda\phi^{\ast}(s/\lambda)$.
  So the worst case distribution is $\mathbb{P}^{\ast}(\tbz=\hbz_{n})=
  \exp(\frac{l(\bt, \hbz_{n})-\eta}{\lambda})\hat{\mathbb{P}}(\tbz=\hbz_{n})$.
  According to \cite{follmer2011stochastic}, the minimizor of 
  the right-hand of the equality is $\eta^{\ast}= \lambda\log(
    \mathbb{E}_{\hat{
  \mathbb{P}}}\left[\exp\left(l(\bt, \tbz)/\lambda\right)
  \right])$, which can be 
  obtained by setting the deviation to 0. Take $\eta^{\ast}$ into the right-hand 
  expression, we have the following  
  \begin{equation}\label{tiledlossequivalence}
  \sup_{\mathbb{P}\ll\hat{\mathbb{P}}}\{\mathbb{E}_{\mathbb{P}}[
  l(\tbz, \bt)]-\lambda D(\mathbb{P}\Vert \hat{\mathbb{P}})\}
  =\lambda\log\left(\mathbb{E}_{\hat{\mathbb{P}}}\left[\exp\left(
  l(\bt, \tbz)/\lambda\right)\right]\right)=\hat{R}(\bt, \lambda).
  \end{equation}

  The corresponding optimal distribution $\mathbb{P}^{\ast}(\tbz=\hbz_{n})=
  \frac{\exp(l(\bt, \hbz_{n})/\lambda)}{\mathbb{E}_{\Pemp}[\exp(l(\bt, \tbz)/\lambda)]}
  \Pemp(\tbz=\hbz_{n})$.
\hfill \qedsymbol

\paragraph{Proof for Proposition \ref{prop: mv}}
With \eqref{tiledlossequivalence}, we can begin our discussion from $\hat{R}(\bt, \lambda)$'s sup problem formulation. 
\begin{equation}
  \begin{aligned}
    &\displaystyle\sup_{\mathbb{P}\ll\hat{\mathbb{P}}}\left\{
      \mathbb{E}_{\mathbb{P}}[l(\bt, \tbz)]-D_{\phi}
    (\mathbb{P}\Vert \hat{\mathbb{P}}) \right\}\\
    =&\displaystyle\sup_{\mathbb{P}\ll\hat{\mathbb{P}}}
    \left\{\mathbb{E}_{\mathbb{P}}[l(\bt, \tbz)]-D_{\phi}
    (\mathbb{P}\Vert \hat{\mathbb{P}})-\mathbb{E}_{\mathbb{P}}
    [\mathbb{E}_{\hat{\mathbb{P}}}[l(\bt, \tbz)]] \right\}\\
    &+\mathbb{E}_{\hat{\mathbb{P}}}[l(\bt, \tbz)]\\
    =&\displaystyle\inf_{\eta}\sup_{\mathbb{P}}\left\{ \eta+
    \mathbb{E}_{\hat{\mathbb{P}}}[\frac{d\mathbb{P}}{d
    \hat{\mathbb{P}}}(l(\bt, \tbz)-\eta-\mathbb{E}_{\hat{\mathbb{P}}}
    [f(\bt, \tbz)])-\lambda\phi(\frac{d\mathbb{P}}{d\hat{\mathbb{P}}})]
    \right\}\\
    &+\mathbb{E}_{\hat{\mathbb{P}}}[l(\bt, \tbz)]\\
    =&\displaystyle\inf_{\eta}\left\{ \eta+\lambda\mathbb{E}_{
      \hat{\mathbb{P}}}[\phi^{\ast}(\frac{l(\bt, \tbz)-
      \eta-\mathbb{E}_{\mathbb{P}}[l(\bt, \tbz)]}{\lambda})]\right\}\\
    &+\mathbb{E}_{\hat{\mathbb{P}}}[l(\bt, \tbz)]
\end{aligned}
\end{equation}
The first equality holds due to the fact that $\mathbb{E}_{\hat{\mathbb{P}}}
[l(\bt, \tbz)]$ is a constant. The second equality holds due to the reason
that it is a lagrange dual expression where $\eta$ is dual variable. 
The third equality holds due to $\phi^{\ast}(s)=\sup_{x}\{x^{\top}s-\phi(s)\}=\exp(s)-1$. The Taylor's expansion of $\phi^{\ast}(s)$ around 
0 is $\phi^{\ast}(s)= s+\frac{1}{2}s^{2}+o(s^{2})$.
For a very large positive $\lambda$, we have: 
\begin{equation}
    \begin{aligned}
        &\displaystyle\inf_{\eta}\left\{ \eta+\lambda\mathbb{E}_{\hat{\mathbb{P}}}[\phi^{\ast}(\frac{l(\bt, \tbz)-\eta-\mathbb{E}_{\hat{\mathbb{P}}[l(\bt, \tbz)]}}{\lambda})]\right\}\\
        =&\displaystyle\inf_{\eta}\{\eta +\lambda\mathbb{E}_{\hat{\mathbb{P}}}[(\frac{l(\bt, \tbz)-\eta-\mathbb{E}_{\hat{\mathbb{P}}}[l(\bt, \tbz)]}{\lambda})\\
        &+\frac{1}{2}(\frac{l(\bt, \tbz)-\eta-\mathbb{E}_{\hat{\mathbb{P}}}[l(\bt, \tbz)]}{\lambda})^{2}+o(\frac{1}{\lambda^{2}})]\}\\
        =&\inf_{\eta}\left\{\frac{1}{2\lambda}\mathbb{E}_{\hat{\mathbb{P}}}\left(l(\bt, \tbz)-\eta-\mathbb{E}_{\hat{\mathbb{P}}}[l(\bt, \tbz)]\right)^{2}\right\}+o(\frac{1}{\lambda^{2}})\\
        \geq&\frac{1}{2\lambda}\mathbb{E}_{\hat{\mathbb{E}}}\left[l(\bt, \tbz)-\mathbb{E}_{\hat{\mathbb{P}}}[l(\bt, \tbz)]\right]^{2}+o(\frac{1}{\lambda^{2}})\\
        =&\frac{1}{2\lambda}\mathbb{V}_{\hat{\mathbb{P}}}[l(\bt, \tbz)]+o(\frac{1}{\lambda^{2}})
      \end{aligned}
\end{equation}

The first equality is Taylor's expansion. The inequality holds because
$\mathbb{E}_{\hat{\mathbb{P}}}[l(\bt, \tbz)]=\arg\min_{x}
\mathbb{E}_{\hat{\mathbb{P}}}[l(\bt, \tbz)-x]^{2}$ then the 
minimum is achieved when $\eta=0$.
\hfill \qedsymbol

Above discussion demonstrates the relationship between $\hR$ and mean-variance when $\lambda$ is sufficient large. When we set our target $\tau$ as a number which is a little larger than the minimal value 
of Empirical Risk Minimization, a feasible $\lambda$ to problem 
\eqref{Prob: klrs} must be a large number. We discuss the problem under the following two assumptions below.

\paragraph{Proof of Proposition \ref{prop: probability inequality}}
\begin{equation}
    \begin{aligned}
    \hat{\mathbb{P}}(l(\bt, \tbz)\geq \tau+\alpha)&=
    \hat{\mathbb{P}}\left(\exp(l(\bt, \tbz)/\lambda)
    \geq \exp((T+\alpha)/\lambda)\right)\\
    &\leq \frac{\mathbb{E}_{\hat{\mathbb{P}}}[
      \exp(l(\bt, \tbz)/\lambda)]}{\exp((\tau+\alpha)/\lambda)}\\
    &\leq \frac{\exp(\tau/\lambda)}{\exp((\tau+\alpha)/\lambda)}=
    \exp(\frac{-\alpha}{\lambda}).
    \end{aligned}
  \end{equation}
  The first inequality holds due to Markov Inequality. The second inequality 
  holds because $(\bt, \lambda)$ is a feasible solution of problem(\ref{Prob: klrs Sim}). 
\hfill \qedsymbol

Particularly when $(\bt, \lambda)$ is the optimal solution of problem \ref{Prob: klrs Sim} which makes the constraint active, the above inequality is a sharp inequality. The inequality
can not be tighter if no other assumptions are made. This is because, in this case the above inequality is as tight as Markov Inequality while Markov Inequality is a sharp inequality.

\paragraph{Proof of Theorem \ref{thm: hierachicalquivalence}}
\begin{equation}
  \begin{aligned}
  &\mathbb{E}_{\mathbb{P}_{\tbz, \tbg}}\left[l(\bt, \tbz)\right]
  \leq \tau+\lambda_{1}D(\mathbb{P}_{\tbg}\Vert \Pemp_{\tbg})
  +\lambda_{2}\mathbb{E}_{\mathbb{P}_{\tbg}}D(\mathbb{P}_{\tbz\vert\tbg}
  \Vert\Pemp_{\tbz\vert\tbg}), \forall\;\; \mathbb{P}_{\tbz, \tbg}\ll\Pemp_{\tbz, \tbg}\\
  \leftrightarrow&\sup_{\mathbb{P}_{\tbz\vert\tbg}\ll\Pemp_{\tbz\vert\tbg}}
  \mathbb{E}_{\mathbb{P}_{\tbg}}\left[\mathbb{E}
  _{\Pemp_{\tbz\vert 
  \tbg}}[l(\bt, \tbz)]-\lambda_{2}D(\mathbb{P}
  _{\tbz\vert\tbg}
 \Vert\Pemp_{\tbz\vert\tbg})
  \right]\\
  &\leq \tau+\lambda_{1}D(\mathbb{P}
  _{\tbg}\Vert\Pemp_{\tbg}), \forall\;\;  \mathbb{P}_{\tbg}\ll\Pemp_{\tbg}\\
  \leftrightarrow&\mathbb{E}_{\mathbb{P}_{\tbg}}\left[\lambda_{2}\log
  \left(\mathbb{E}_{\Pemp_{\tbz\vert\tbg}}
  \exp\left(f(\bt, \tbz)/\lambda_{2}\right)\right) \right]
  \leq \tau +\lambda_{1}D(\mathbb{P}
  _{\tbg}\Vert\Pemp_{\tbg}), \forall\;\;  \mathbb{P}_{\tbg}\ll\Pemp_{\tbg}\\
  \leftrightarrow&\sup_{\mathbb{P}_{\tbg}\ll\Pemp_{\tbg}}
  \mathbb{E}_{\mathbb{P}_{\tbg}}\left[\lambda_{2}\log\left(
  \mathbb{E}_{\Pemp_{\tbz\vert\tbg}}
  \exp\left(l(\bt, \tbz)/\lambda_{2}\right)\right) 
  -\lambda_{1}D(\mathbb{P}_{\tbg}\Vert\Pemp_{\tbg})\right]\leq \tau\\
  \leftrightarrow&\lambda_{1}\log\left(\mathbb{E}_{\Pemp_{\tbg}}
  \left[ \exp(\lambda_{2}\log\left(
    \mathbb{E}_{\Pemp_{\tbz\vert\tbg}}
    \exp\left(l(\bt, \tbz)/\lambda_{2}\right)\right)/\lambda_{1})\right]
  \right)\leq \tau
\end{aligned}
\end{equation}
The first and third $\leftrightarrow$ are due to the inequality holding for 
any distribution within the support.

The second and third $\leftrightarrow$ hold for the equality \ref{tiledlossequivalence}.
\hfill \qedsymbol

In practical applications, people often do not simultaneously address 
shifts in group and individual. Many works assume that there is no 
distribution shift happens to $\tbz\vert\tbg$ 
\cite{sagawa2019distributionally, zhang2020coping, arjovsky2019invariant, 
duchi2023distributionally}. Under this assumption we have $D(\mathbb{P}_{\tbz\vert\tbg}\Vert\Pemp_{\tbz\vert\tbg})=0$ and the optimal value of
\eqref{eq: hierachicalKL-RS} is achieved when $\lambda_{2}=0$.
In this case, our \eqref{eq: hierachicalKL-RS} will degenerate into 
Group KL-RS formulation defined as following:

\begin{definition}\textit{Group KL-RS}

  \begin{equation}\label{groupKL-RS}
    \begin{aligned}
      &\min_{\bt\in\Theta, \lambda\geq 0}\lambda\\
      &\text{s.t.}\lambda\log\left(
        \mathbb{E}_{\Pemp_{\tbg}}\exp\left(
        \mathbb{E}_{\Pemp_{\tbz\vert \tbg}}
        f(\bt, \tbz)/\lambda\right)\right)\leq T.
    \end{aligned}
  \end{equation}
\end{definition}

\section{Proofs and Details for Section \ref{sec: alg}}
\label{app: alg}
\subsection{Solving KL-RS}
\label{app: solving KL-RS}
We present our solving process in Algorithm \ref{alg: solving KL-RS}. 
Our algorithm will involve a total of $T$ rounds of iteration. 
At iteration $t$, we first fix $\bt_{t-1}$ and query Algorithm \ref{alg: bisection}
to obtain $\lambda_{t}$. Then we fix $\lambda_{t-1}$ and query 
gradient based Algorithm \ref{alg: nnupdate} to obtain $\bt_{t}$. 
Particularly our gradient update procedure starts from $\bt_{t-1}$ 
instead of a random guess. This approach allows us to leverage the 
results of previous gradient descents, avoiding the need for a complete 
optimization from scratch and saving significant computational costs. 
This method is similar to Continuation strategy for solving LASSO problem, 
which will gradually increase the coefficient of the regularization. This 
method is very similar to the continuation strategy used to solve Lasso 
problems. In this strategy, the regularization term weight gradually 
increases, and optimization continues from the previously obtained 
parameters after the weight change\cite{allgower2012numerical}.

First, we will discuss the optimization of $\lambda$. We set $\lambda$ within a \
range $[\lambda_{l}, \lambda_{u}]$, where $\lambda_{u}>\lambda_{l}>0$. 
We set the lower bound for two reasons. Firstly, because this paper considers a 
nontrivial KL-RS, excluding the case where $\lambda=0$ is feasible. 
Secondly, to avoid numerical errors in calculations when $\lambda$ is very close 
to 0. We set an upper bound because during normal training of neural networks, 
losses typically have an upper limit. Beyond a certain point, increasing $\lambda$
has negligible effects on the computation due to the limitations of computer 
precision.

\IncMargin{1em} % 使得行号不向外突出 
\begin{algorithm}\label{alg: solving KL-RS}
    \SetAlgoNoLine % 不要算法中的竖线
    \SetKwInOut{Input}{\textbf{Input}}\SetKwInOut{Output}{\textbf{Output}} % 替换关键词
    \Input{
        initial guess $\bt_{0}$, $\lambda_{0}=\lambda_{u}$, 
        target performance $\tau$, maximum iteration $T$,
        \\}

    \Output{
        $\bt_{T}$, $\lambda_{T}$;
        }
    \BlankLine
    \For{$t=1$ to $T$}{
      Query Algorithm (\ref{alg: bisection}) to obtain $\lambda_{t}$;\\
      Query Algorithm (\ref{alg: nnupdate}) to obtain $\bt_{t}$;\\
    }
    \caption{Solving KL-RS}
\end{algorithm}
\DecMargin{1em}

\IncMargin{1em} % 使得行号不向外突出 
\begin{algorithm}\label{alg: bisection}
    \SetAlgoNoLine % 不要算法中的竖线
    \SetKwInOut{Input}{\textbf{Input}}\SetKwInOut{Output}{\textbf{Output}} % 替换关键词
    \Input{
        fixed parameter $\bt_{t-1}$, Interval $[\lambda_{l}, \lambda_{u}]$, 
        target performance $\tau$, maximum searching iteration $I$,
        batch size $B$\\}
    \Output{$\lambda_{I}$;}
    \BlankLine
    Sample $B$ samples $\{\hbz_{n}\}_{n\in[B]}$;\\
    \If{$\frac{1}{B}\sum_{n\in[B]}l(\bt, \hbz_{n})>\tau$}{
      $\lambda_{I}=\lambda_{u}$;\\
    }
    \Else{
    Let $\overline{\lambda}=\lambda_{u}$ and $
    \underline{\lambda}=\lambda_{l}$;\\
    \For{$i=1$ to $I$}{      
      Let $\lambda_{i}=\frac{\overline{\lambda}+\underline{\lambda}}{2}$;\\
      \If{$\lambda_{i}\log(\frac{1}{B}\displaystyle{\sum_{n\in[B]}}
      \exp(l(\hbz_{n}, \bt_{t-1})/\lambda_{i}))<\tau$}{
        $\overline{\lambda}=\lambda_{i}$;\\
      }
      \Else{
        $\underline{\lambda}=\lambda_{i}$;\\
      }
    }
  }
    \caption{Bisection Search at iteration $t$}
\end{algorithm}
\DecMargin{1em}

\IncMargin{1em} % 使得行号不向外突出 
\begin{algorithm}\label{alg: nnupdate}
    \SetAlgoNoLine % 不要算法中的竖线
    \SetKwInOut{Input}{\textbf{Input}}\SetKwInOut{Output}{\textbf{Output}} % 替换关键词
    \Input{
        fixed $\lambda_{t}$, an input $\bt_{t-1}$, target performance $\tau$, 
        maximum iteration $I$,
        batch size $B$,  step size $\gamma_{i}$\\}

    \Output{
        $\bt_{t, I}$;
        }
    \BlankLine
    Let $\bt_{t, 0}=\bt_{t-1}$;\\
    \For{$i=1$ to $I$}{
      Sample $B$ samples $\{\hbz_{i, n}\}_{n\in[B]}$;\\
      Update $\bt_{t, i}=\bt_{t, i-1}-\gamma_{i}\nabla_{\bt}\displaystyle{
        \sum_{n\in[B]}}g_{t}(\bt_{t, i-1}, \hbz_{i, n})$
    }
    \caption{$\bt$ Updating for KL-RS at  $t$}
\end{algorithm}
\DecMargin{1em}

Then we discuss the optimization procedure of $\bt$. We can directly apply a 
gradient based algorithm to optimize problem \eqref{exp: 1}.
And $g_{t}(\bt, \tbz)$ can inherent various excellent properties of $l(\bt, \tbz)$, 
such as convexity, lipschitz continuous and lipschitz smooth as following statement:

This implying that using any gradient based algorithm to solving $\min_{\bt\in\Theta}\mathbb{E}_{\Pemp}[f(\bt, \tbz; \lambda)]$
dose not result in much additional computational overhead compared to solving \eqref{Prob: eop}. 
In fact, they enjoy the same order of convergence speed with only different 
constants. However, it is noteworthy that when $\lambda$ is very small,
these constants can increase significantly, which implies that the optimization
may also suffer from some difficulties.

As for why we do not directly optimize
\begin{equation}
    \min_{\bt\in\Theta}\mathbb{E}_{\hat{\mathbb{P}}}[\exp(\frac{l(\tbz, 
    \bt)}{\lambda_{t}})], 
\end{equation}
the main reason is that the magnitude of the gradient $\nabla\exp(\frac{l(\tbz,
 \bt)}{\lambda_{t}})=\exp(\frac{l(\bt, \tbz)}{\lambda_{t}})\frac{\nabla l(\tbz, 
 \bt)}{\lambda_{t}}$ is influenced by the value $l(\bt, \tbz)$, and as the 
 gradient proceeds and the loss changes, the optimization process become unstable.

Since we adopt gradient based algorithm from an initial $\bt_{t-1}$ 
which satisfies $\hat{R}(\bt_{t-1}, \lambda_{t})\leq \tau$.
This statement holds due to $\lambda_{t}$ is a output of Algorithm \ref{alg: bisection}. Optimizing 
Dividing by $\exp(\tau/\lambda_{t})$ 
can be seen to a certain extent, as normalizing.

\subsection{Solving Hierarchical KL-RS}
\label{app: solving hierarchicalKL-RS}

\begin{equation}
\hat{F}_{t}(\bt)\triangleq\frac{1}{L}\sum_{\ell\in[L]}\hat{G}_{t}(\bt, \hbg_{\ell})
\end{equation}

\begin{equation}
\hat{G}_{t}(\bt, \hbg_{\ell})\triangleq q_{t}(\frac{1}{M}\sum_{m\in[M]}f_{t}(\bt, \hbz_{\ell, m}))
\end{equation}

\begin{equation}
\nabla\hat{F}_{t}(\bt)=\frac{1}{L}\sum_{\ell\in[L]}\nabla\hat{G}_{t}(\bt, \hbg_{\ell})
\end{equation}

\begin{equation}
\nabla\hat{G}_{t}(\bt, \hbg_{\ell})=\nabla q_{t}(\frac{1}{M}\sum_{m\in[M]}f_{t}(\bt, \hbz_{\ell, m}))/M\sum_{m\in[M]}\nabla f_{t}(\bt, \hbz_{\ell, m})
\end{equation}

\IncMargin{1em} % 使得行号不向外突出 
\begin{algorithm}\label{alg: solvinghierachicalKL-RS}
    \SetAlgoNoLine % 不要算法中的竖线
    \SetKwInOut{Input}{\textbf{Input}}\SetKwInOut{Output}{\textbf{Output}} % 替换关键词
    \Input{
        initial guess $\bt_{0}$, $\lambda_{1}^{0}=\lambda_{u}$, 
        $\lambda_{2}^{0}=\lambda_{u}$, 
        target performance $T$, maximum outer iteration $T$,
        \\}

    \Output{
        $\bt_{T}$, $\lambda_{T}$;
        }
    \BlankLine
    \For{$s=1$ to $T$}{
      Query Algorithm (\ref{alg: bisectionhierarchical}) to 
      obtain $(\lambda_{1}^{t}, \lambda_{2}^{t})$;\\
      Query Algorithm (\ref{alg: nnupdatehierarchical}) to obtain $\bt_{t}$;\\
    }
    \caption{Solving Hierarchical KL-RS}
\end{algorithm}
\DecMargin{1em}

\IncMargin{1em} % 使得行号不向外突出 
\begin{algorithm}\label{alg: bisectionhierarchical}
    \SetAlgoNoLine % 不要算法中的竖线
    \SetKwInOut{Input}{\textbf{Input}}\SetKwInOut{Output}{\textbf{Output}} % 替换关键词
    \Input{
        fixed parameter $\bt_{t-1}$, Interval $[\lambda_{l}, \lambda_{u}]$, 
        target performance $\tau$, coefficient $w\geq 0$, maximum searching iteration $I$, 
        group level batch size $L$, individual level batch size $M$\\}
    \Output{$(\lambda_{1}^{I}, \lambda_{2}^{I})$;}
    \BlankLine
    Sample $L$ samples $\{\hbg_{\ell}\}_{\ell\in[L]}$ from $\tbg$;\\
    \For{$\ell=1$ to $L$}{
      Sample $M$ samples $\{\hbz_{\ell, m}\}_{m\in[M]}$ from 
      $\tbz\vert \hbg_{\ell}$;\\
    }
    \If{$\frac{1}{LM}\displaystyle\sum_{\ell\in[L], m\in[M]}l(\bt_{t-1}, 
    \hbz_{\ell, m})>\tau$}{
      Let $(\lambda_{1}^{I}, \lambda_{2}^{I})=(\lambda_{u}, \lambda_{u})$;\\
    }
    \Else{
    Let $\alpha_{l}^{0}=\lambda_{l}$, $\alpha_{u}^{0}=\lambda_{u}$,
    $\lambda_{1}^{0}=\lambda_{u}$ and $\lambda_{2}^{0}=\lambda_{u}$;\\
    \For{$i=1$ to $I$}{
      Update $\beta_{l}^{i}=\frac{1}{3}[2\alpha_{l}^{(i-1)}+
      \alpha_{u}^{(i-1)}]$ and $\beta_{u}^{i}=\frac{1}{3}
      [\alpha_{l}^{(i-1)}+2\alpha_{u}^{(i-1)}]$;\\
      Query Algorithm to obtain $\zeta_{l}^{i}$ and $\zeta_{u}^{i}$ respectively;\\
      \If{$\beta_{l}^{i}+w\zeta_{l}^{i}\leq 
      \beta_{u}^{i}+w\zeta_{u}^{i}$}{
        Update $(\alpha_{l}^{i}, \alpha_{u}^{i})=(\beta_{l}^{i}, 
        \alpha_{u}^{(i-1)})$;\\
        \If{$\beta_{l}^{i_{1}}+w\zeta_{l}^{i}\leq \lambda_{1}^{(i-1)}
        +w\lambda_{2}^{(i-1)}$}{
           Update $(\lambda_{1}^{i}, \lambda_{2}^{i})=(\beta_{l}^{i}, \zeta_{l}^{i})$
        }
        \Else{
          Update $(\lambda_{1}^{i}, \lambda_{2}^{i})=(\lambda_{1}^{(i-1)}, 
          \lambda_{2}^{(i-1)})$
        }
      }
      \Else{
        Update $(\alpha_{l}^{i}, \alpha_{u}^{i})=(\alpha_{l}^{(i-1)}, 
        \beta_{u}^{(i)})$;\\
        \If{$\beta_{u}^{i_{1}}+w\zeta_{u}^{i}\leq \lambda_{1}^{(i-1)}
        +w\lambda_{2}^{(i-1)}$}{
           Update $(\lambda_{1}^{i}, \lambda_{2}^{i})=(\beta_{u}^{i}, \zeta_{u}^{i})$
        }
        \Else{
          Update $(\lambda_{1}^{i}, \lambda_{2}^{i})=(\lambda_{1}^{(i-1)}, 
          \lambda_{2}^{(i-1)})$
        }
      }
    }
  }
    \caption{Bisection Search for Hierarchical KL-RS}
\end{algorithm}
\DecMargin{1em}

\IncMargin{1em} % 使得行号不向外突出 
\begin{algorithm}\label{alg: bisectiondown}
    \SetAlgoNoLine % 不要算法中的竖线
    \SetKwInOut{Input}{\textbf{Input}}\SetKwInOut{Output}{\textbf{Output}} % 替换关键词
    \Input{
        fixed parameter $\bt$, fixed parameter $\beta$, Interval $[\lambda_{l}, \lambda_{u}]$, 
        target performance $\tau$, maximum searching iteration $I$,
        given samples $\{\hbg_{\ell}, \hbz_{\ell, m\in[M]}\}_{\ell\in[L]}$, }
    \Output{$\zeta_{I}$;}
    \BlankLine
    \If{$\beta\log(\frac{1}{L}\sum_{\ell\in[L]}\exp(\frac{\sum_{m\in[M]}
    l(\bt, \hbz_{\ell, m})}{M\beta}))>\tau$}{
      $\zeta_{I}=\lambda_{u}$;\\
    }
    \Else{
    Let $\overline{\zeta}=\lambda_{u}$ and $
    \underline{\zeta}=\lambda_{l}$;\\
    \For{$i=1$ to $I_{2}$}{      
      Let $\zeta_{i}=\frac{\overline{\zeta}+\underline{\zeta}}{2}$;\\
      \If{$ \hat{F}_{\beta, \zeta_{i}}(\bt)< 1 
      $}{
        $\overline{\zeta}=\zeta_{i}$;\\
      }
      \Else{
        $\underline{\zeta}=\zeta_{i}$;\\
      }
    }
  }
    \caption{Bisection Search for $\zeta$}
\end{algorithm}
\DecMargin{1em}

We present our solving process in Algorithm \ref{alg: solvinghierachicalKL-RS}.
The overall optimization process of Algorithm \ref{alg: solvinghierachicalKL-RS} 
is similar to Algorithm \ref{alg: solvingKL-RS}. But Algorithm \ref{alg: bisectionhierarchical}
and Algorithm \ref{alg: nnupdatehierarchical} are much more difficult than
Algorithm \ref{alg: bisection} and Algorithm \ref{alg: nnupdate}.

Firstly, let us clarify why \eqref{exp: 2} is equivalent to $\min_{\bt\in\Theta}
\hat{R}(\bt, \lambda_{t1}, \lambda_{t2})$. 
\begin{equation}
  \begin{aligned}
  &\exp(\hat{R}(\bt, \lambda_{1}^{t}, \lambda_{2}^{t})/\lambda_{1}^{t})/
  \exp(\tau/\lambda_{1}^{t})\\
  =&\left(\mathbb{E}_{\tbg}
  \left[ \exp\left(\lambda_{2}^{t}\log\left(
    \mathbb{E}_{\tbz\vert\tbg}
    \exp\left(l(\bt, \tbz)/\lambda_{2}^{t}\right)\right)/\lambda_{1}^{t}
    \right)\right]
  \right)/\exp(\tau/\lambda_{1}^{t})\\
  =&\Ex_{\tbg}\left[\exp\left(\frac{\lambda_{2}^{t}}{\lambda_{1}^{t}}\log\left(
    \Ex_{\tbz\vert\tbg}\exp(l(\bt, \tbz)/\lambda_{2}^{t})
  \right)-\tau/\lambda_{1}^{t}\right)\right]\\
  =&\Ex_{\tbg}\left[\exp\left(\frac{\lambda_{2}^{t}}{\lambda_{1}^{t}}\log\left(
    \Ex_{\tbz\vert\tbg}\exp(l(\bt, \tbz)/\lambda_{2}^{t})/\exp(\tau/\lambda_{2}^{t})
  \right)\right)\right]\\
  =&\Ex_{\tbg}\left[\left[\Ex_{\tbz\vert\tbg}\exp(\frac{l(\bt, \tbz)-
  \tau}{\lambda_{2}^{t}})
  \right]^{\frac{\lambda_{2}^{t}}{\lambda_{1}^{t}}}\right]\\
  =&\mathbb{E}_{\tbg}[
    q_{t}(\mathbb{E}_{\tbz\vert \tbg}f_{t}(\bt, \tbz))]=F_{t}(\bt)
  \end{aligned}
\end{equation}

Then, we discuss the optimization for $(\lambda_{1}^{t}, \lambda_{2}^{t})$. We can 
still use Bisection Search Algorithm but adopt a little modification. 
We have the following proposition 
\begin{proposition}
For a given $\bt\in\Theta$, \eqref{exp: 2} is convex optimization
with respect to $(\lambda_{1}, \lambda_{2})$.
\end{proposition}
\begin{proof}
  $\lambda_{1}+k\lambda_{2}$ is convex with respect to $(\lambda_{1}, \lambda_{2})$.
  So, to prove our statemet, we only need to prove the feasible set is also convex.
  From the proof procedure \ref{proof: hierachicalquivalence}, we have the following:
  \begin{equation}
    \begin{aligned}
    &\lambda_{1}\log\left(\mathbb{E}_{\Pemp_{\tbg}}
    \left[ \exp(\lambda_{2}\log\left(\mathbb{E}_{\Pemp_{\tbz\vert\tbg}}
      \exp\left(l(\bt, \tbz)/\lambda_{2}\right)\right)/\lambda_{1})\right]
    \right)\leq \tau\\
    \leftrightarrow&\sup_{\mathbb{P}\ll\hat{\mathbb{P}}}\{
      \mathbb{E}_{\mathbb{P}}[l(\bt, \tbz)]-\lambda_{1}D(\mathbb{P}_{\tbg}\Vert \Pemp_{\tbg})
      -\lambda_{2}\mathbb{E}_{\mathbb{P}_{\tbg}}D(\mathbb{P}_{\tbz\vert\tbg}
      \Vert\Pemp_{\tbz\vert\tbg})
    \} \leq \tau.
    \end{aligned}
  \end{equation}
  For a given $\mathbb{P}\ll\Pemp$, $
    \mathbb{E}_{\mathbb{P}}[l(\bt, \tbz)]-\lambda_{1}D(\mathbb{P}_{\tbg}\Vert \Pemp_{\tbg})
    -\lambda_{2}\mathbb{E}_{\mathbb{P}_{\tbg}}D(\mathbb{P}_{\tbz\vert\tbg}
    \Vert\Pemp_{\tbz\vert\tbg})$ is simply a linear function of
    $(\lambda_{1}, \lambda_{2})$. Taking pointwise $\sup$ to linear function will obtain 
    a convex function, so the feasible set is also convex.
\end{proof}

Thanks to the convexity of the problem and having only two variables, we can 
still use a search based algorithm  to optimize $(\lambda_{1}, \lambda_{2})$.
For ease of describing our searching algorithm, we define the following 
expression:
\begin{equation}
  \hat{F}_{\lambda_{1}, \lambda_{2}}(\bt)\triangleq \frac{1}{L}
  \sum_{\ell\in[L]}q_{\lambda_{1}, \lambda_{2}}(
  \frac{1}{M}\sum_{m\in[M]}f_{\lambda_{2}}(\bt, \hbz_{\ell, m})).
\end{equation}
where $f_{\lambda_{2}}(\bt, \tilde{\bz})\triangleq\exp(\frac{l(\bt, \tbz)-\tau}
{\lambda_{2}})$ and $q_{\lambda_{1}, \lambda_{2}}(x)\triangleq 
x^{\frac{\lambda_{2}}{\lambda_{1}}}$.

Algorithm \ref{alg: bisectionhierarchical} and Algorithm \ref{alg: bisectiondown}
demonstrate our search approach. The basic idea is that, for a given $\lambda_{1}$, we 
can use binary search to find the optimal $\lambda_{2}$.

\iffalse
The gradient of $F(\bt)$ is given by 
\begin{equation}
    \nabla_{\bt} F(\bt) = \mathbb{E}_{\tbg}\left[ 
      (\mathbb{E}_{\tbz\vert \tbg}[\nabla_{\bt} f_{s}(\bt, \tbz)])^{\top}
      \nabla_{\bt} q_{\lambda_{1}, \lambda_{2}}(\mathbb{E}_{\tbz\vert\tbg}
      [f(\bt, \tbz)])
    \right].
\end{equation}

To construct a biased gradient estimator, we can i.i.d sample
$L$ samples $\{\hbg\}_{\ell\in[L]}$ from distribution $\tbg$.
Then for each $\hbg_{\ell}$, we i.i.d sample $M$ samples $\{\hbz_{\ell, m}\}_{m\in[M]}$
from conditional distribution $\tbz\vert\hbg_{\ell}$.
Then our gradient estimator has the following form:
\begin{equation}
\nabla_{\bt} \hat{F}_{s}(\bt, \{\hbg_{\ell}, \hbz_{\ell, m\in[M]}
\}_{\ell\in[L]})\triangleq\frac{1}{L}\sum_{\ell\in[L]}
\nabla_{\bt}\hat{F}_{s}(\bt, \{\hbg_{\ell}, \hbz_{\ell, m\in[M]}\}).
\end{equation}

\begin{equation}
  \nabla_{\bt}\hat{F}_{s}(\bt, \{\hbg_{\ell}, \hbz_{\ell, m\in[M]}\})\triangleq 
  (\frac{1}{M}\sum_{m\in[M]}\nabla_{\bt} f_{s}(\bt, \hbz_{\ell, m}))^{\top}
  \nabla_{\bt} q_{s}(\frac{1}{M}\sum_{m\in[M]}f_{s}(\bt, \hbz_{\ell, m})).
\end{equation}

Above is the gradient of an objective such that:
\begin{equation}
\begin{aligned}
\hat{F}_{s}(\bt, \{\hbg_{\ell}, \hbz_{\ell, m\in[M]}\}_{\ell\in[L]})
&\triangleq \frac{1}{L}\sum_{\ell\in[L]}\hat{F}_{s}(\bt, \hbg_{\ell}, 
\hbz_{\ell, m\in[M]}),\\
\hat{F}_{s}(\bt, \{\hbg_{\ell}, \hbz_{\ell, m\in[M]}\})&\triangleq
q_{s}(\frac{1}{M}\sum_{m\in[M]}f(\bt, \hbz_{\ell, m})).
\end{aligned}
\end{equation}
\fi

Proof for proposition \ref{prop: preconvergence}
\begin{proof}
  The Lipschitz smoothness property of the $q_{t}(x)$ can be easily 
  demonstrated. It is sufficient to note that, under the conditions where 
  Assumption \ref{blf} holds and non-negative $(\lambda_{1}^{t}, \lambda_{2}^{t})$, 
  the function $f_{t}(\bt, \tbz)$ is bounded within interval $[\exp(\frac{-\tau}
  {\lambda_{2}^{t}}), \exp(\frac{C_{0}-T}{\lambda_{2}^{t}})]$. The input of 
  $q_{t}(x)$ is also within this non-negative interval. Considering that the 
  $q_{t}(x)$ is a power function with a positive exponent, it is lipschitz smooth
  within this interval. We can assume this coefficient as $S_{q_{t}}$
   
  When assumption \ref{stronglyconvex} holds, 
  $\hat{G}_{t}(\bt, \hbg_{\ell})$ is $\mu_{t}$-strongly convex, 
  when assumption \ref{lipsmooth} holds, $\hat{G}_{t}(\bt, \hbg_{\ell})$ 
  is $S_{f}$ smooth. This statement can be easily verified using similar
  process as the proof of Proposition \ref{inherent}. W.l.o.g, 
  we can assume the coefficients as $\mu_{t}$ and $S_{f}$ respectively.

\end{proof}

Next, we discuss the optimization for $\bt$. We will give the convergence guarantee
for Algorithm \ref{alg: nnupdatehierarchical}. In the subsequent discussion, we
omit the subscript $t$.

Let $\sigma_{g}^{2}\triangleq \sup_{\hbg\in\mathcal{G}, \bt\in\Theta}
\mathbb{E}_{\tbz\vert \hbg}\Vert f(\bt, \tbz)
-\mathbb{E}_{\tbz\vert\hbg}f(\bt, \tbz)\Vert^{2}_{2}$.
Then under assumption \ref{blf}, $\sigma_{g}^{2}<+\infty$ which mean 
the random variable $f(\bt, \tbz)$ has bounded variance.

In our algorithm, at update step $i$, we generate $\{\hbg_{i, \ell\in[L]}\}$
from distribution of $\tbg$. For $\tbg_{i, \ell}$, we sample 
$\{\hbz_{i, \ell, m\in[M]}\}$ from the conditional distribution $\tbz
\vert\tbg$. In fact, such a sampling process can be viewed as a discrete random process 
that is independently and identically distributed at each moment.  We use 
$\{\{\hbg_{i, \ell}, \hbz_{i, \ell, m\in[M]}\}_{\ell\in[L]}
\}_{i\in[I]}$ to denote this sampling random process. 

We define the following auxiliary functions to help our
convergence analysis:
\begin{equation}
  \begin{aligned}
  \hat{p}(\bt, \hbg_{i, \ell\in[L]})&\triangleq\frac{1}{L}\sum_{\ell\in[L]}
  \hat{p}(\bt, \hbg_{i, \ell});\\
  \hat{p}(\bt, \hbg_{i, \ell})&\triangleq q(\frac{1}{M}\sum_{m\in[M]}
  f(\hbz_{i, \ell, m}, \bt)).
  \end{aligned}
\end{equation}
\begin{proof}
Let $\bt^{\ast}\in\arg\displaystyle\min_{\bt\in\Theta}F(\bt)$ and 
$A_{i}=\frac{1}{2}\Vert \bt_{i}-\bt^{\ast}\Vert_{2}^{2}$. $A_{i}$ is 
actually a random variable because the sampling process is random, and hence
$\bt_{i}$ generated by the algorithm is also random. We do not focus
on its support set and distribution, but only focus on its mean value 
$a_{i}\triangleq \mathbb{E} A_{i}$ which is taking expectation over the 
random process $\{\{\tbg_{i, \ell}, \tbz_{i, \ell, m\in[M]}\}_{\ell\in[L]}
\}_{i\in[I]}$. Of course, this value is independent of the sampling after time 
$s$. In the following discussion, there will be a considerable amount of 
expectation calculations. For the sake of formula simplicity, we will denote 
them uniformly as $\mathbb{E}$, but will specify what the expectation is taken 
over near the formulas.

Since projection operator $\Pi_{\Theta}(\cdot)$
is non-expansive, we can conclude
\begin{equation}
  \begin{aligned}
    A_{i+1}&=\frac{1}{2}\Vert \bt_{i+1}-\bt^{\ast}\Vert_{2}^{2}\\
    &=\frac{1}{2}\Vert \Pi_{\Theta}(\bt_{i}-\gamma_{i}\nabla_{\bt}
    \hat{p}(\bt_{i}, \hbg_{i, \ell\in[L]})-\Pi_{\Theta}(\bt^{\ast}))
    \Vert_{2}^{2}\\
    &\leq\frac{1}{2}\Vert \bt_{i}-\bt^{\ast}-\gamma_{i}\nabla_{\bt}
    \hat{p}(\bt_{i}, \hbg_{i, \ell\in[L]})\Vert_{2}^{2}\\
    &=A_{i}+\frac{1}{2}\gamma_{i}^{2}\Vert\nabla_{\bt}\hat{p}(\bt_{i}, 
    \hbg_{i, \ell\in[L]})\Vert_{2}^{2}-\gamma_{i}\nabla_{\bt}
    \hat{p}(\bt_{i}, \hbg_{i, \ell\in[L]})^{\top}(\bt_{i}-\bt^{\ast}).
  \end{aligned}
\end{equation}

The equality hold due to the definition. The inequality holds due to 
projection operator is non-expansive.

The following discussion is conducted under the condition where $\bt_{i}$
is given.
Dividing $\gamma_{i}$ on both sides and taking expectation over 
$\{\tbg_{i, \ell}, \tbz_{i, \ell, m\in[M]}\}_{\ell\in[L]}$, the
following holds
\begin{equation}\label{exp: 6}
  \mathbb{E}\nabla_{\bt}\hat{p}(\bt_{i}, \hbg_{i, \ell\in[L]})
  ^{\top}(\bt_{i}-\bt^{\ast})\leq \frac{A_{i}-\mathbb{E}[A_{i+1}
  \vert \bt_{i}]}{\gamma_{i}}+\frac{1}{2}\gamma_{i}\mathbb{E}\Vert 
  \nabla_{\bt}\hat{p}(\bt_{i}, \tbg_{i, \ell\in[L]})\Vert_{2}^{2}.
\end{equation}
When $\bt_{i}$ is given $A_{i}$ is also given. Since $\hat{p}(\bt_{i}, 
\tbg_{i, \ell})$ is $\mu$-strongly convex, then we have 
\begin{equation}
  \begin{aligned}
  &-\nabla_{\bt}\hat{p}(\bt_{i}, \tbg_{i, \ell})^{\top}(\bt_{i}
  -\bt^{\ast})\leq \hat{p}(\bt^{\ast}, \tbg_{i, \ell})-
  \hat{p}(\bt_{i}, \tbg_{i, \ell})-\frac{\mu}{2}\Vert \bt_{i}
  -\bt^{\ast}\Vert_{2}^{2}\\
  =&\underbrace{\hat{p}(\bt^{\ast}, \tbg_{i, \ell})-p(\bt^{\ast}, 
  \tbg_{i, \ell})}_{\triangleq \zeta_{i, \ell, 1}}
  +\underbrace{p(\bt^{\ast}, \tbg_{i, \ell})-p(\bt_{i}, 
  \tbg_{i, \ell})}_{\triangleq \zeta_{i, \ell, 2}}\\
  &+\underbrace{p(\bt_{i}, \tbg_{i, \ell})- \hat{p}(\bt_{i},
   \tbg_{i, \ell})}_{\triangleq \zeta_{i, \ell, 3}}
  -\frac{\mu}{2}\Vert \bt_{i}-\bt^{\ast}\Vert_{2}^{2},\forall \ell.
  \end{aligned}
\end{equation}

Taking expectation over $\{\tbg_{i, \ell}, \tbz_{i, \ell, m\in[M]}\}$
on both sides, by the definition of $p(\bt, \tbg_{i, \ell})$, it holds 
$\mathbb{E}[\zeta_{i, \ell, 2}\vert \bt_{i}]=
\mathbb{E}_{\tbg_{i, \ell}}[\zeta_{i, \ell, 2}\vert \bt_{i}]=
\mathbb{E}_{\tbg_{i, \ell}}[F({\bt^{\ast}})-F(\bt_{i})\vert \bt_{i}]
=F(\bt^{\ast})-F(\bt_{i})$,
then 
\begin{equation}\label{exp: 4}
  -\mathbb{E}[\nabla_{\bt}\hat{p}(\bt_{i}, \tbg_{i, \ell})^{\top}
  (\bt_{i}-\bt^{\ast})]\leq \mathbb{E}\zeta_{i, \ell, 1}+\mathbb{E}
  \zeta_{i, \ell, 3}+F(\bt^{\ast})-F(\bt_{i})-\mu A_{i}.
\end{equation}

Recall that $\bt^{\ast}$ and $\bt_{i}$ are independent of $\{\tbg_{i, \ell},
\tbz_{i, \ell, m\in[M]}\}$. 
Define 
\begin{equation}
    \Delta_{q}(M)=\frac{S_{q}\sigma_{g}^{2}}{2M}.
\end{equation}

Then according to \cite{hu2020sample}, we have the following proposition
\begin{proposition}\label{prop: 1}
  For a sample $\tbg$ and $M$ i.i.d. samples $\{\tbz\}_{m\in[M]}$ from conditional 
  distribution $\hat{\mathbb{P}}(\tbz\vert\tbg)$, and a $\bt\in\Theta$
  which is independent of $\tbg$ and $\{\tbz\}_{m\in[M]}$, we have
  \begin{equation}
    \vert \mathbb{E}_{\tbg, \tbz_{m\in[M]}}\hat{p}(\bt, 
    \tbg, \tbz_{m\in[M]})-F(\bt)\vert\leq \nabla_{q}(M).
  \end{equation}
\end{proposition}
Then we can conclude 
\begin{equation}
  \begin{aligned}
    \vert\zeta_{i, \ell, 1}\vert\leq \Delta_{q}(M);\\
    \vert\zeta_{i, \ell, 3}\vert\leq \Delta_{q}(M).
  \end{aligned}
\end{equation}
With the above inequality and  \eqref{exp: 4}, we have
\begin{equation}\label{exp: 9}
  -\mathbb{E}[\nabla_{\bt}\hat{p}(\bt_{i}, \tbg_{i, \ell})^{\top}
  (\bt_{i}-\bt^{\ast})]\leq 2\Delta_{q}(M)+F(\bt^{\ast})
  -F(\bt_{i})-\mu A_{i}, \forall \ell\in[L].
\end{equation}
Then with \eqref{exp: 9} we can obtain the following
\begin{equation}\label{exp: 5}
  \begin{aligned}
&\mathbb{E}_{\tbg_{i, \ell\in[L]}, \tbz_{i, (\ell, m)\in[L, M]}}\nabla_{\bt}\hat{p}(\bt_{i}, \tbg_{i, \ell\in[L]})^{\top}
(\bt_{i}-\bt^{\ast})\\
=&\frac{1}{L}\sum_{\ell\in[L]}\mathbb{E}_{\tbg_{i, \ell}, \tbz_{i, \ell, m\in[M]}}
\nabla_{\bt}\hat{p}(\bt_{i}, \tbg_{i, \ell})^{\top}(\bt_{i}
-\bt^{\ast})\\
\geq& \frac{1}{L}\sum_{\ell\in[L]}[-2\Delta_{q}(M)
+F(\bt_{i})-F(\bt^{\ast})]+\mu A_{i}\\
=&-2\Delta_{q}(M)
+F(\bt_{i})-F(\bt^{\ast})+\mu A_{i}.
  \end{aligned}
\end{equation}

Summing up \eqref{exp: 6} and \eqref{exp: 5}, we obtain
 \begin{equation}\label{exp: 10}
    F(\bt_{i})-F(\bt^{\ast})\leq 2\Delta_{q}(M)-\mu A_{i}
    +\frac{A_{i}-\mathbb{E}[A_{i+1}\vert \bt_{i}]}{\gamma_{i}} +\frac{1}{2}\gamma_{i}\mathbb{E}
    \Vert \nabla_{\bt}\hat{p}(\bt_{i}, \tbg_{i, \ell\in[L]})\Vert_{2}^{2}, 
 \end{equation}
where the expectation is taking over $\{\tbg_{i, \ell}, 
\tbz_{i, \ell, m\in[M]}\}_{\ell\in[L]}$.
Recall that $\hat{\bt}_{I}=\frac{1}{I}\sum_{i\in[I]}\bt_{i}$, we have
\begin{equation}\label{exp: 8}
\mathbb{E}[F(\hat{\bt}_{I})-F(\bt^{\ast})]=\mathbb{E}[F(\frac{1}{I}
\sum_{i\in[I]}\bt_{i})-F(\bt^{\ast})]\leq \frac{1}{S}\sum_{i\in[I]}
\mathbb{E}[F(\bt_{i})-F(\bt^{\ast})],
\end{equation}
where the inequality holds due to the convexity of $F(\bt)$. \eqref{exp: 8}
is taking expectation over random process $\{\{\tbg_{i, \ell}, 
\tbz_{i, \ell, m\in[M]}\}_{\ell\in[L]}\}_{i\in[S]}$.

Since $\nabla_{\bt}\hat{p}(\bt_{i}, \tbg_{i, \ell\in[L]})$ is 
$\mu$-strongly convex and $S_{F}$-Lipschitz smooth, we have
\begin{equation}\label{exp: 11}
  \begin{aligned}
    \begin{aligned}
      \mathbb{E}\|\nabla_{\bt} \hat{F}(\bt)\|_2^2 & \leq 2 \mathbb{E}\left\|
      \nabla_{\bt} \hat{F}(\bt)-\nabla_{\bt} \hat{F}\left(\bt^*\right)\right\|_2^2
      +2 \mathbb{E}\left\|\nabla_{\bt} \hat{F}\left(\bt^*\right)\right\|_2^2 \\
      & \leq 2 S^2\left\|\bt-\bt^*\right\|_2^2+2 \mathbb{E}\left\|\nabla_{\bt}
      \hat{F}\left(\bt^*\right)\right\|_2^2 \\
      & \leq 4 S^2 / \mu\left(F(\bt)-F\left(\bt^*\right)\right)+2
       \mathbb{E}\left\|\nabla_{\bt} \hat{F}\left(\bt^*, 
       \{\tbg_{\ell}, \tbz_{\ell, m\in[M]}\}_{\ell\in[L]}\right)\right\|_2^2,
      \end{aligned}
  \end{aligned}
\end{equation}
where the expectation is taking over $\{\tbg_{\ell}, 
\tbz_{\ell, m\in[M]}\}_{\ell\in[L]}$. With \eqref{exp: 10} and \eqref{exp: 11},
we can obtain:

\begin{equation}
  \begin{aligned}
  F(\bt_{i})-F(\bt^{\ast})\leq& 2\Delta_{q}(M)-\mu A_{i}
  +\frac{A_{i}-\mathbb{E}[A_{i+1}\vert \bt_{i}]}{\gamma_{i}} \\
  &+ \frac{1}{2}\gamma_{i}(4S_{F}^{2}/\mu
  (F(\bt)-F(\bt^{\ast}))+2\mathbb{E}\Vert \nabla_{\bt}\hat{F}(\bt^{\ast},
  \{\tbg_{i, \ell}, \tbz_{i, \ell, m\in[M]}\}_{\ell\in[L]})
  \Vert_{2}^{2}).
  \end{aligned}
\end{equation}

We use $\hat{F}_{i}(\bt^{\ast})$ to denote $\hat{F}(\bt^{\ast},
\{\tbg_{i, \ell}, \tbz_{i, \ell, m\in[M]}\}_{\ell\in[L]})$. 
Set $\gamma_{i}=\frac{1}{\mu(i+c)}$ and $c=\max\{4S_{F}^{2}/\mu^{2}-1, 0\}$.
It is east to verify that $\gamma_{i}\leq \gamma_{1}\leq \frac{\mu}{4S_{F}^{2}}$.
Therefore, we have:
\begin{equation}\label{exp: 7}
  \begin{aligned}
F(\bt_{i})-F(\bt^{\ast})\leq& \frac{1}{1-2\gamma_{i}S_{F}^{2}/\mu}
(2\Delta_{q}(M)-\mu A_{i}
+\frac{A_{i}-\mathbb{E}[A_{i+1}\vert \bt_{i}]}{\gamma_{i}}+\gamma_{i}\mathbb{E}\Vert \nabla_{\bt}\hat{F}_{i}
(\bt^{\ast})\Vert_{2}^{2})\\
&\leq 2(2\Delta_{q}(M)-\mu A_{i}
+\frac{A_{i}-\mathbb{E}[A_{i+1}\vert \bt_{i}]}{\gamma_{i}}
+\gamma_{i}\mathbb{E}\Vert \nabla_{\bt}\hat{F}_{i}
(\bt^{\ast})\Vert_{2}^{2}).
  \end{aligned}
\end{equation}

Taking expectation over the random process $\{\{\tbg_{i, \ell}, 
\tbz_{i, \ell, m\in[M]}\}_{\ell\in[L]}\}_{i\in[I]}$, with \eqref{exp: 7} we have
\begin{equation}
  \begin{aligned}
      & \frac{1}{I} \sum_{i\in[I]} \mathbb{E}\left[F\left(\bt_i\right)
      -F\left(\bt^*\right)\right] \\
      \leq & \frac{2}{I} \sum_{i\in[I]}\left[\mathbb{E}_{\bt_{i}}\left[2 \Delta_q\left(M\right)
      -\mu A_i+\frac{A_i-\mathbb{E}[A_{i+1}\vert \bt_{i}]}{\gamma_i}+\gamma_i \mathbb{E}\left\|\nabla 
      \hat{F}_{i}\left(\bt^*\right)\right\|_2^2\right]\right] \\
      = &\frac{2}{I}\sum_{i\in[I]}\left[ 2\delta_{q}(M)-\mu a_{i}+\frac{a_{i}-a_{i+1}}
      {\gamma_{i}}+\gamma_{i}\mathbb{E}\Vert \nabla_{\bt}\hat{F}_{i}(\bt^{\ast})\Vert_{2}^{2}\right]\\
      = & \frac{2}{I} \sum_{i\in[I]}\left[2 \Delta_q\left(M\right)+\gamma_i
       \mathbb{E}\left\|\nabla \hat{F}\left(\bt^*\right)\right\|_2^2\right]
       +\frac{2}{I} \sum_{i=2}^I a_t\left(\frac{1}{\gamma_i}-\frac{1}{\gamma_{i-1}}
       -\mu\right)+\frac{2}{I} a_1\left(\frac{1}{\gamma_1}-\mu\right)\\
      \leq & \frac{2}{I} \sum_{i\in[I]}\left[2 \Delta_q\left(M\right)+\gamma_i 
      \mathbb{E}\left\|\nabla \hat{F}\left(\bt^*\right)\right\|_2^2\right]+
      \frac{2}{I} \sum_{i=2}^I a_t\left(\frac{1}{\gamma_i}-\frac{1}{\gamma_{i-1}}
      -\mu\right)+\frac{2}{I} a_1\frac{1}{\gamma_1}\\
      = & \frac{2}{I} \sum_{i\in[I]}\left[2 \Delta_q\left(M\right)+\gamma_i 
      \mathbb{E}\left\|\nabla \hat{F}\left(\bt^*\right)\right\|_2^2\right]
      +\frac{S_{F}^{2}}{4\mu I}\Vert \bt_{1}-\bt^{\ast}\Vert_{2}^{2}.
    \end{aligned}
\end{equation}
The first inequality holds due to \eqref{exp: 7}. The first equality holds due to
the definition of $a_{i}$ and the tower property of conditional expectation 
$\mathbb{E}[A_{i+1}]=\mathbb{E}_{\bt_{i}}[A_{i+1}\vert \bt_{i}]$. 
The second equality is a simply rearranging. The second inequality holds due to
omitting negative term $-\frac{2\mu a_{1}}{I}$. The last equality holds due to the
definition of $\gamma_{i}$.

With \eqref{exp: 8}, we can obtain:
\begin{equation}
\mathbb{E}\left[F(\hat{\bt}_{I})-F(\bt^*)\right] 
\leq \frac{4}{I} \sum_{i\in[I]} \Delta_q(M)+\frac{1}{I} 
\sum_{i\in[I]} \frac{2 \mathbb{E}\Vert\nabla \hat{F}_{i}\left(\bt^*\right)
\Vert_{2}^{2}}{\mu(i+c)}+\frac{S_F^2}{4 \mu I}\left\|\bt_1-\bt^*\right\|_2^2.
\end{equation}
Since the random process $\{\{\tbg_{i, \ell}, 
\tbz_{i, \ell, m\in[M]}\}_{\ell\in[L]}\}_{i\in[I]}$ is strictly stationary
stochastic process, we let $\mathbb{E}\Vert \nabla_{\bt}\hat{F}(\bt^{\ast})
\Vert_{2}^{2}=\mathbb{E}\Vert \nabla_{\bt}\hat{F}_{1}(\bt^{\ast})
\Vert_{2}^{2}=\cdots= \mathbb{E}\Vert \nabla_{\bt}\hat{F}_{I}(\bt^{\ast})
\Vert_{2}^{2}$.
With a classical inequality $\sum_{i\in[I]}\frac{1}{s+c}\leq \sum_{i\in[I]}\frac{1}{s}
\leq \log(I)+1$, we can obtain
\begin{equation}\label{exp: 12}
  \mathbb{E}\left[F(\hat{\bt}_{I})-F(\bt^*)\right] \leq 
  \frac{4}{I} \sum_{i\in[I]} \Delta_q(M)+\frac{2 \mathbb{E}
  \Vert\nabla \hat{F}\left(\bt^*\right)\Vert_{2}^{2}(\log (I)+1)+S_F^2 /
   4\Vert\bt_1-\bt^*\Vert_{2}^{2}}{\mu I}.
\end{equation}
\end{proof}
Although $L$ dose not apper explicitly in the convergence result 
\eqref{exp: 12}, $L$ actually will affect the value $\mathbb{E}\Vert \nabla_{\bt}
\hat{F}(\bt^{\ast})\Vert_{2}^{2}$. $\mathbb{E}\Vert \nabla_{\bt}
\hat{F}(\bt^{\ast})\Vert_{2}^{2}$ is the second moment of gradient
estimator. With a larger $L$, the variance will be smaller. Thus, 
we can trade off between the total number of iterations and the computational 
complexity within single iteration by adjusting $L$.

\subsection{Hyperparameters Tuning}
\label{sec: hyperparameter tuning}
In this section, we will demonstrate the convenicen of KL-RS in
parameter tuning. 

Compared to the radius $r$ in DRO and the tilted factor $\lambda$ in 
$\hat{R}(\bt, \lambda)$, our taeget performance $\tau$ is a 
more explicitly meaningful hyperparameter enabling decision maker to
make better selection. 

Our target performance $\tau$ is a natural quality which can be linked
to other quantities in the optimization problem. In other words,
$T$ can be set as a function of certain quantities, and adjusted by 
tuning coefficients within the function.

\cite{long_robust_2023} normalize $\tau$ by $E$ where they let 
$T=aE$ with $a\geq 1$. Then they tune $a$ to tune $T$ without
the need to spend effort on exvessive consideration of the loss 
distribution. 

However, this method only considers the feasibility of $\tau$ ignoring the
loss spread information. In fact, we do not know what magnitude of $a$ 
qualifies as "sufficiently large". For example, when $\max_{i\in[N]}l(\tbz, 
\bt_{N}^*)-\min_{i\in[N]}l(\tbz, \bt_{N}^*)
\leq 0.001\mathbb{E}_{\Pemp}[l(\bt, \tbz)]$, recall that $\bt_{N}^*$ is the optimal solution of \eqref{Prob: eop}, even $a=1.01$ is a too large value.

To address this issue, we can introduce some loss spread
information into our function to adjust target performance $\tau$. 

One possible choice could be $T=a\max_{i\in[N]}f(\tbz, \hat{\bt})
+(1-a)\min_{i\in[N]}f(\tbz, \hat{\bt})$ where $0\leq a\leq 1$. When 
we $a$ is larger, $T$ is larger and we will obtain a more robust model.
It is worth noting that we need to ensure that $a$ is large enought to
ensure $T\geq E$ to make \eqref{2} have feasible solution.

Inspired from theorem (\ref{meanvariance}), another possible choice could
be $T=E+a\mathbb{V}_{\hat{\mathbb{P}}}[f(\tbz, \hat{\bt})]$
where $a\geq 0$. Since $\tau$ increase with $a$, when 
we increase $a$ we will obtain a more robust model. Compared to the 
previously mentioned approach, this method ensures that the selected 
$T$ always produce a feasible \eqref{2}.

When applying KL-RS in practice, we can combine the aforementioned 
approach with cross-validation to select the parameters.

\subsubsection{Compare with tilted factor}

\cite{li_tilted_nodate, li_tilted_2021, qi2022attentional} directly
use $\hat{R}(\bt,\lambda)$ as optimization objective for their machine
learning tasks and call this optimization problem \textit{Tilted Loss Risk Minimization (TERM)}
. They tune $\lambda$ to obtain model with different levels of 
robustness; a smaller $\lambda$ will yiled a more robust model. Although
the trend of model's performance with respect to $\lambda$ is known, it is
still necessary to select $\lambda$ by cross-validation in practice. Although
possessing similar optimization structures, our KL-RS exhibits superior
performance in determeing hyperparameters.

On one hand, $\lambda$ is a relatively abstract concept, making it difficult for 
decision-makers to intuitively determine the appropriate range for 
$\lambda$. However, decison maker may have initial performance expectation or can
easily derive a target $\tau$ from the results of ERM.

On other hand, the hyperparameters determined by KL-RS through cross-validation
tend to exhibit more stability compare to TERM. Similar phenomena are also mentioned
when the statistic distance is wasserstein distance \cite{long_robust_2023}. 
To validate our claims, we conducted experiments on the HIV1 dataset.

We select the last 10$\%$ of the dataset as the test set, while the remaining
samples are used for training. We randomly divide train set into five parts and
then conducted 5 fold cross validation and get the best hyperparameter. We repeat 
this process 4 times with different random seeds. In KL-RS we adopt line 
search to find the best target $\tau$. In TERM, we employ geometric search to
find the best tilted factor $\lambda$. We adopt different search methods
because $\tau$ appears as an addictive term in KL-RS, while $\lambda$ appears 
as a multiplier in TERM. The experiments demonstrate that these two
search methods are effective. Our principle for selecting the 
best parameters is to choose the parameter that result in the 
highest accuracy for positives on the validation part. The selected 
parameters are displayed in table (\ref{table: cross-validate}).

We take the average of selected as target $\tau$ and tilted factor $\lambda$ to 
train KL-RS and TERM respectively and display the results in table (\ref{table: crossvalperf}).

\begin{table*}[t]
  \centering
  \caption{5-fold-cross-validation to select best hyperparameter}
  \label{table: cross-validate}
  \begin{tabular}{|c|c|c|c|c|c|c|c|c|}
    \hline
    \multicolumn{1}{|c|}{\multirow{3}{*}{Fold}}&\multicolumn{4}{c|}{KL-RS}&\multicolumn{4}{c|}{TERM}\\
    \cline{2-9}
    &\multicolumn{4}{c|}{Seed}&\multicolumn{4}{c|}{Seed}\\
    \cline{2-9}
    &\multicolumn{1}{c|}{\multirow{1}{*}{0}} &\multicolumn{1}{c|}{\multirow{1}{*}{1}}
    &\multicolumn{1}{c|}{\multirow{1}{*}{2}} &\multicolumn{1}{c|}{\multirow{1}{*}{3}}
    &\multicolumn{1}{c|}{\multirow{1}{*}{0}} &\multicolumn{1}{c|}{\multirow{1}{*}{1}}
    &\multicolumn{1}{c|}{\multirow{1}{*}{2}} &\multicolumn{1}{c|}{\multirow{1}{*}{3}}\\
    \hline
    0&0.21&0.205&0.205&0.215&64&64&64&45.12\\
    \hline
    1&0.21&0.205&0.215&0.215&32&11.28&22.56&45.12\\
    \hline
    2&0.21&0.2&0.205&0.21&45.12&64&45.12&45.12\\
    \hline
    3&0.2&0.2&0.21&0.205&11.28&45.12&32&32\\
    \hline
    4&0.215&0.205&0.21&0.215&64&64&45.12&64\\
    \hline
    \end{tabular}
    
\end{table*}

\begin{table*}[t]
  \centering
  \caption{Performance with selected parameter}
  \label{table: crossvalperf}
  \begin{tabular}{|c|c|c|c|c|c|c|c|}
    \hline
    Obj& Parameter & Positive Acc & Negative Acc & Acc\\
    \hline
    KL-RS& 0.209 & $\mathbf{0.923_{0.009}}$ & $0.921_{0.004}$ & $0.924_{0.001}$\\
    \hline
    TERM & 43.28 & $0.917_{0.012}$ & $0.927_{0.004}$ & $0.924_{0.002}$\\
    \hline
    KL-RS& 0.209 & $\mathbf{0.923_{0.009}}$ & $0.921_{0.004}$ & $0.924_{0.001}$\\
    \hline
    TERM & 49.68 & $0.917_{0.012}$ & $0.925_{0.004}$ & $0.923_{0.002}$\\
    \hline
    KL-RS & 0.203 & $0.909_{0.016}$ & $0.930_{0.005}$ & $0.925_{0.002}$\\
    \hline
    TERM & 41.76 & $\mathbf{0.917_{0.012}}$ & $0.927_{0.004}$ & $0.924_{0.002}$\\ 
    \hline
    KL-RS & 0.212 & $\mathbf{0.922_{0.009}}$ & $0.921_{0.004}$ & $0.921_{0.003}$\\
    \hline
    TERM & 46.27 & $0.917_{0.012}$ & $0.925_{0.004}$ & $0.924_{0.002}$\\
    \hline
    \end{tabular}

\end{table*}

Furthermore, the fixed setting of $\lambda$ throughout the 
entire process in TERM may not be very suitable for neural 
networks. Similar to our KL-RS, TERM puts more weights on harder
samples to robustify a model. Consider two samples, the harder
one's loss is $l_{1}$ while the easier one's loss is $l_{2}$
with $l_{1}> l_{2}$. TERM gives $\exp(\frac{l_{1}-l_{2}}{\lambda})$
times more weights to harder sample compare to easier sample. 
One characteristic of gradient-based optimization algorithms 
is that the loss decreases continuously as the iterations 
progress.  Empirical evidence suggests that the loss at the 
beginning and end of training often differs by an order of 
magnitude. In this case, when we choose a small $\lambda$, 
large losses may pose a risk of numerical overflow at the 
initial stages of training. When we choose a large $\lambda$, 
TERM can not robustify a model by assigning harder sample more
weight in later stages of training. Based on the above analysis, in principle, adaptively adjusting the value of $\lambda$ during the gradient descent process according to the sample losses can be beneficial for the training process. \cite{qi_attentional-biased_2023}
also demonstrates through experiments that gradually decreasing $\lambda$ over multiple stages can improve the algorithm's performance. However, multi-stage adjustment of $\lambda$ introduces additional considerations during the implementation of the algorithm,
\emph{i.e.} when should we adjust $\lambda$? what value should $\lambda$ be adjusted to? 

Our KL-RS optimization process is naturally an adaptive multi-stage TERM. We do not need to consider these additional issues, as our $\lambda$ adjusts adaptively based on the current loss and our target $\tau$.

\section{Limitations}
\label{app: limi}
Our paper does not discuss the case of using more general $\phi$ divergences. The main reason is that when using general $\phi$ divergence, we cannot obtain a reformulation similar to \eqref{Prob: klrs Sim}. This necessitates simultaneously optimizing both the distribution and the parameter $\bt$. The exploration of more general $\phi$-divergences might be a direction for future research.

Additionally, our research makes minimal assumptions about the true distribution $\Popt$, leading to relatively general conclusions. When our KL-RS framework is applied to specific problems, the true distribution may exhibit more definite characteristics, such as a normal distribution or a Bernoulli distribution. In these cases, the expression of our problem might be further simplified and presented in a more insightful mathematical form.
Exploring whether KL-RS can yield more insightful conclusions in more specific machine learning tasks compared to general cases might be a direction for future research.

\section{Potential Society Impacts}
\label{app: impacts}
We believe our work will have a positive social impact. More researchers will pay attention to the potential applications of the RS framework, which focuses on target-oriented robust optimization, in machine learning. Especially for high-risk task scenarios, our KL-RS framework might offer robust solutions. Adjusting the KL-RS framework based on specific application scenarios will further enrich the framework's content and generate insights beyond those mentioned in this paper.
